# Supplementary material for: ReFACTor: Practical Low-Rank Matrix Estimation Under Column-Sparsity
Source: arXiv:1705.07654 ancillary file (2017-05-22)
Supplement: Supplementary file 1 [file SI.pdf]

# Supporting Information for "*ReFACTor*: Practical Low-Rank Matrix Estimation Under Column-Sparsity"

## 1 Additional Proofs

**Proof of Theorem 2.** By the proof of Theorem 1, under the assumptions, with high probability *ReFACTor* correctly identifies the active columns, in other words $[\hat{X}_t^{RF}]_j = [X]_j = 0$ for $j > t$, and $[\hat{X}_t^{RF}]_j = [\hat{X}_1]_j$ for $j \le t$. Thus, w.h.p,

$$\left|\left|\hat{X}_1 - X\right|\right|_F^2 - \left|\left|\hat{X}_t^{RF} - X\right|\right|_F^2 = \sum_{j=t+1}^{n} ||y\mathbf{u}v_j||^2 = y^2 \sum_{j=t+1}^{n} v_j^2 \,.$$

By Lemma 5, it is enough to show that with high probability $\sum_{j=t+1}^n v_j^2 \ge 1 - \frac{t+\log n}{n}(1+\epsilon)$. Indeed, by Lemma 1, we can write

$$v_j^2 = \frac{\tilde{w}_j^2}{\sum_{j=1}^n \tilde{w}_j^2},$$

where $\tilde{\mathbf{w}} \sim \mathcal{N}(0, I - \mathbf{b}\mathbf{b}^\top)$, or equivalently, $\tilde{\mathbf{w}} = \mathbf{z} - \mathbf{b}\mathbf{b}^\top\mathbf{z}$, where $\mathbf{z} \sim \mathcal{N}(0, I_n)$. It is easy to verify that $\|\tilde{\mathbf{w}}\|^2 \sim \chi^2_{n-1}$ since $\mathbf{b}$ is a unit vector (see also proof of Lemma 1). Similarly, since the $t$-dimensional vector $(b_1, \ldots, b_t)$ is a unit vector then $\sum_{i=1}^t \tilde{w}_i^2 \sim \chi^2_{t-1}$ Thus, by Lemma 6, with high probability,

$$\sum_{j=1}^{t} \tilde{w}_j^2 \le (t + \log n)(1 + \epsilon/4),$$

$$\sum_{j=1}^{n} \tilde{w}_j^2 \ge (n-1)(1 - \epsilon/4)$$

Thus, with high probability,

$$\sum_{j=t+1}^{n} v_j^2 \ge 1 - \frac{t + \log n}{n}(1 + \epsilon)$$

□

We now prove the Lemmas (for convenience we also state them again).

**Lemma 1. Marginal distribution of the entries of w.** Let $w_j$ be the $j$-th entry of $\mathbf{w}$ from (8), namely the projection of $\mathbf{v}$ on $\mathbf{b}^\perp$. Let $\tilde{\mathbf{w}} \sim \mathcal{N}(0, I - \mathbf{b}\mathbf{b}^\top)$. Then for $j = 1, \ldots n$, $w_j$ has the same distribution as

$$\frac{\tilde{w}_j}{\sqrt{\sum_{j=1}^n \tilde{w}_j^2}}$$

and $\sum_{j=1}^n \tilde{w}_j^2 \sim \chi^2_{n-1}$.

**Proof of Lemma 1.** Due to symmetry, $\mathbf{w}$ is a random vector uniformly distributed on the sphere orthogonal to $\mathbf{b}$. Let $P = I - \mathbf{b}\mathbf{b}^\top$ be the projection matrix to the hyperplane perpendicular to $\mathbf{b}$. Let $\mathbf{z} \sim \mathcal{N}(\mathbf{0}, I_n)$ be a vector of i.i.d. standard Gaussians, and $\tilde{\mathbf{w}} = P\mathbf{z}$ its projection. Then, $\mathbf{w}$ may be generated as $\mathbf{w} = \tilde{\mathbf{w}}/\|\tilde{\mathbf{w}}\|$. By using $P^\top P = P$, we have $\tilde{\mathbf{w}} \sim \mathcal{N}(\mathbf{0}, P)$. Therefore, $\tilde{w}_j \sim \mathcal{N}(0, 1 - b_j^2)$. Let $B$ be an orthonormal matrix whose first column is $\mathbf{b}$. Then, $B\tilde{\mathbf{w}} \sim \mathcal{N}(\mathbf{0}, BPB^\top) = \mathcal{N}(\mathbf{0}, \mathrm{diag}(0, 1, \ldots, 1))$. Therefore, $\|\tilde{\mathbf{w}}\|^2 = \|B\tilde{\mathbf{w}}\|^2 \sim \chi^2_{n-1}$.

□

**Lemma 2. Right singular vector is small in inactive columns.** Let $j > t$ and $\alpha > 1$. Then

$$Pr\left\{v_j^2 > \frac{s^2\alpha^2\log(n)}{n}\right\} \le \frac{2}{n^{\alpha^2/2}}\,.$$

**Proof of Lemma 2.** Let $\alpha \ge 1$. For $j > t$, we have $b_j = 0$, giving $\tilde{w}_j \sim \mathcal{N}(0,1)$, and

$$Pr(\tilde{w}_j > \frac{\alpha}{2}\sqrt{\log n}) \le \exp(-\alpha^2\log n/8) = n^{-\alpha^2/8},$$

using a normal tail bound [2]. Similarly, as $\|\tilde{\mathbf{w}}\|^2 \sim \chi^2_{n-1}$, using the tail bound $Pr(\chi^2_k < zk) \le (ze^{1-z})^{k/2}$ [2], for a large enough $n$,

$$Pr(\|\tilde{\mathbf{w}}\|^2 < n/4) \le n^{-\alpha^2/8}.$$

Since $v_j = s\tilde{w}_j/\|\tilde{\mathbf{w}}\|$ for $j > t$,

$$\begin{aligned} &Pr\left(\frac{\tilde{w}_j^2}{\|\tilde{\mathbf{w}}\|^2} > \frac{\alpha^2\log n/4}{n/4}\right) \\ =&Pr\left(v_j^2 > s^2\cdot\frac{\alpha^2\log n}{n}\right) \le 2n^{-\alpha^2/8}. \end{aligned}$$

□

**Lemma 3. Right singular vector is large in active columns.** Let $j \le t$ and $\alpha > 1$. Assume that

$$b_j^2 \ge \frac{4s^2\alpha^2\log(n)}{c^2 n}\,.$$

Then

$$Pr\left\{v_j^2 < \frac{s^2\alpha^2\log(n)}{n}\right\} \le \frac{2}{n^{\alpha^2/8}}\,.$$

**Proof of Lemma 3.** By the assumption $b_j^2 > (4s^2\alpha^2\log(n))/(c^2n)$, in the event that $w_j^2 < \alpha^2\log(n)/n$, we have

$$\begin{aligned} v_j^2 &= (cb_j + sw_j)^2 \\ &> \left(c|b_j| - s\alpha\sqrt{\log(n)/n}\right)^2 > s^2\alpha^2\log(n)/n\,. \end{aligned}$$

It follows that

$$\begin{aligned} \Pr\left\{v_j^2 < s^2\frac{\alpha^2\log(n)}{n}\right\} &\le \Pr\left\{w_j^2 > \alpha^2\frac{\log(n)}{n}\right\} \\ &\le \frac{2}{n^{\alpha^2/2}}\,, \end{aligned}$$

where the last inequality follows from a normal tail bound [2]. □

**Lemma 4. A lower bound on the cosine.** Let $x > \sqrt{1+2\sqrt{\beta}}$. Then with high probability $c^2 \ge \frac{1}{2}$.

**Proof of Lemma 4.** Note that on the one hand, by expanding $Y = y\mathbf{u}\mathbf{v}^\top$ we get

$$\mathbf{b}^\top Y^\top Y\mathbf{b} = y^2\langle\mathbf{b},\mathbf{v}\rangle^2 = y^2c^2 \quad (1)$$

$$\mathbf{w}^\top Y^\top Y\mathbf{w} = y^2\langle\mathbf{w},\mathbf{v}\rangle^2 = y^2s^2 \quad (2)$$

and on the other hand, by expanding $Y = X + Z/\sqrt{n}$ we get

$$\mathbf{b}^\top Y^\top Y\mathbf{b} = x^2 + \frac{2}{\sqrt{n}}X^\top Z + \frac{1}{n}\mathbf{b}^\top Z^\top Z\mathbf{b} \quad (3)$$

$$\mathbf{w}^\top Y^\top Y\mathbf{w} = \mathbf{w}^\top Z^\top Z\mathbf{w}/n\,. \quad (4)$$

where we have used $\mathbf{w} \perp \mathbf{b}$ to obtain the latter equality. Note that $\mathbf{b}^\top Z^\top Z\mathbf{b} \sim \chi^2_m$, and $X^\top Z \sim N(0, x^2)$. By Lemma 6, with high probability $(Z\mathbf{b})^\top(Z\mathbf{b}) \geq (1-\epsilon/2)m$. By the tail of the normal distribution, with high probability $X^\top Z \geq -x \log n$. Thus, with high probability $y^2c^2 \geq x^2 + (1-\epsilon)\beta$.

Let $\sigma_1$ denote the top singular value of $Z$, so that $\sigma_1^2 \geq \mathbf{w}^\top Z^\top Z\mathbf{w}$. Combining (2) and (4) we have for any $\varepsilon > 0$

$$\begin{aligned} Pr\left\{y^2s^2 > (1+\sqrt{\beta}+\varepsilon)^2\right\} &\leq Pr\left\{\sigma_1 > 1+\sqrt{\beta}+\varepsilon\right\} \\ &\leq exp\left(-\frac{n\varepsilon^2}{2}\right), \end{aligned}$$

Where the last inequality follows from e.g. Theorem II.13 of [1]. Let $g(\varepsilon) = (1+\sqrt{\beta}+\varepsilon)^2 - (1-\varepsilon)\beta$. Since $g$ is increasing on $\varepsilon > 0$ and $g(0) = 1 + 2\sqrt{\beta} < x^2$, choose $\varepsilon_0 > 0$ such that $x^2 > g(2\varepsilon_0)$. Then $(1+\sqrt{\beta}+2\varepsilon_0)^2 < x^2 + (1-2\varepsilon_0)\beta$, hence

$$\begin{aligned} Pr\left\{c^2 \leq s^2\right\} &= Pr\left\{y^2c^2 \leq y^2s^2\right\} \\ &\leq Pr\left\{y^2s^2 > (1+\sqrt{\beta}+2\varepsilon_0)^2\right\} \\ &+ Pr\left\{y^2c^2 < x^2 + (1-2\varepsilon_0)\beta\right\} \\ &\leq 2\cdot exp\left(-\frac{(2\varepsilon_0)^2 n\beta}{4}\right) \\ &= 2\cdot exp\left(-\varepsilon_0^2 n\beta\right). \end{aligned}$$

But $y^2 = y^2c^2 + y^2s^2$ hence $c^2 \leq s^2$ is equivalent to $c^2 \leq 1/2$. □

**Lemma 5. A lower bound on the singular value.** Let $x, y$ be defined as above. Then with high probability $y > x$.

**Proof of Lemma 5.** From a variational characterization,

$$y^2 = \mathbf{v}^\top Y^\top Y\mathbf{v} \geq \mathbf{b}^\top Y^\top Y\mathbf{b}$$

By Lemma 6, with high probability $(Z\mathbf{b})^\top(Z\mathbf{b}) \geq (1-\epsilon)m$. By the tail of the normal distribution, with high probability $X^\top Z \leq x \log n$. Thus, with high probability $y^2 \geq \mathbf{b}^\top Y^\top Y\mathbf{b} \geq x^2$. □

**Lemma 6.** Let $X \sim \chi^2_m$. Then, we have $\Pr(X \leq (1-\epsilon)m) \leq e^{-\epsilon^2 m}$. Also, for every $0 < \epsilon < 2$, we have $\Pr(X \geq (1+\epsilon)m) \leq e^{-\epsilon^2 m/8}$.

**Proof of Lemma 6.** Using a $\chi^2$ lower tail bound,

$$Pr(X \leq (1-\epsilon)m) \leq ((1-\epsilon)e^{\epsilon})^{m/2} \leq e^{-m\epsilon^2/2}.$$

Using an upper tail bound, and for $\epsilon < 2$,

$$Pr(X > (1+\epsilon)m) \leq ((1+\epsilon)e^{-\epsilon})^{m/2} \leq e^{-m\epsilon^2/8}.$$

□

**Lemma 7.** Let $w_1, \ldots, w_m \sim \mathcal{N}(0,1)$ be independent standard normal random variables variables, and let $w_{(1)}, \ldots, w_{(m)}$ be their order statistics. Let $\delta > 0$ be a fixed constant. There is a constant $C > 0$, such that for $t \leq (1-\delta)m$, with high probability $w_{(1)}^2 + \ldots + w_{(m-t)}^2 > Cm$.

**Proof of Lemma 7.** Let $F$ be the cumulative distribution function of $\chi^2_1$. Let $p = \frac{m-t}{3m}$, and let $\epsilon = F^{-1}(p)$. Let $X = |\{j \leq m \mid w_j^2 \leq \epsilon\}|$. Now, $X \sim B(m,p)$, and thus, using a Chernoff bound, with high probability $|\{j \leq m \mid w_j^2 \leq \epsilon\}| < 2mp$. Thus, w.h.p

$$w_{(1)}^2 + \ldots + w_{(m-t)}^2 \geq \epsilon(m-t-2mp) \geq \frac{\epsilon\delta m}{3}$$

□

**Claim 1.** For a column $j$, let $T_j^{RF}, T_j^{RF+}$ be the ReFACTor and ReFACTor+ statistics respectively, as previously defined. Then,

$$(T_i^{RF+})^2 = \frac{T_i^{RF}}{\|[Y]_i\|^2}$$

**Proof:**

$$\begin{aligned}
T_i^{RF+} &= \frac{\sum_{j=1}^{r} y_j^2 (v_i)_j^2}{\sqrt{\sum_{j=1}^{m} y_j^2 (v_i)_j^2}\sqrt{\sum_{j=1}^{r} y_j^2 (v_i)_j^2}} \\
&= \sqrt{\frac{\sum_{j=1}^{r} y_j^2 (v_i)_j^2}{\sum_{j=1}^{m} y_j^2 (v_i)_j^2}} = \sqrt{\frac{T_i^{RF}}{\|[Y]_i\|^2}}
\end{aligned}$$

□

We now use this result to show that the theorems hold also for the *ReFACTor+* variant. In order to do so, we first modify the assertions in several Lemmas. Specifically, we prove the following:

**Lemma 8. The *ReFACTor+* score is small for inactive columns.** With high probability, for all $j > t$ we have

$$T_j^{RF+} = \frac{y^2 v_j^2}{\|[Y]_j\|^2} \leq \frac{2y^2 s^2 \beta \log(n)}{n}$$

**Proof of Lemma 8.** We first note that

$$\|[Y]_j\|^2 = x^2 b_j^2 + \frac{1}{n}\|[Z]_j\|^2 + 2\frac{x b_j}{\sqrt{n}}\mathbf{a}[Z]_j$$

Since for $j > t$ we have $b_j = 0$, we have

$$\|[Y]_j\|^2 = \frac{1}{n}\|[Z]_j\|^2$$

Since $\|[Z]_j\|^2 \sim \chi_m^2$, with high probability for all $j > t$ we have

$$\frac{\beta}{2} \leq \|[Y]_j\|^2$$

By Lemma 2

$$Pr\left\{v_j^2 > \frac{2s^2\alpha^2 \log(n)}{\beta n}\right\} \leq \frac{2}{n^{\alpha^2/\beta}}.$$

Thus, the lemma follows by setting $\alpha^2 \geq 2\beta$ and noting that $\|[Y]_j\|^2 \geq \beta/2$. □

**Lemma 9. The *ReFACTor+* score is large for active columns.** Let $C = \max\{\beta(x^2+\beta), 4\}$. With high probability, for all $j \leq t$ such that

$$b_j^2 \geq \frac{s^2 C \log(n)}{c^2 n}.$$

we have

$$T_j^{RF+} = \frac{y^2 v_j^2}{\|[Y]_j\|^2} \geq \frac{2y^2 s^2 \beta \log(n)}{n}$$

**Proof of Lemma 9.** We note that

$$\|[Y]_j\|^2 = x^2 b_j^2 + \frac{1}{n}\|[Z]_j\|^2 + 2\frac{x b_j}{\sqrt{n}}\mathbf{a}[Z]_j$$

and therefore with high probability for all $j \leq t$ we have

$$\|[Y]_j\|^2 \leq 2(x^2 + \beta).$$

Now, by Lemma 3 we have

$$Pr\left\{v_j^2 < \frac{2(x^2+\beta)s^2\alpha^2 \log(n)}{n}\right\} < \frac{2}{n^{-\alpha^2(x^2+\beta)/4}}$$

Thus, by setting $\alpha \geq \max\{\sqrt{2\beta}, \sqrt{\frac{8}{x^2+\beta}}\}$ the Lemma follows. □

**Theorem 4.** *Assume $x > \sqrt{1 + 2\sqrt{\beta}}$, where $\beta = m/n$. There exists a constant $C$ such that if for all $j = 1, \dots, t$ we have*

$$b_j^2 > C \frac{\log(n)}{n},$$

*then, with high probability*

$$\left|\left|\hat{X}_t^{RF+} - X\right|\right|_F^2 \le \left|\left|\hat{X}_1 - X\right|\right|_F^2 .$$

**Proof:** By Lemma 4, with high probability $s^2 \le c^2$. Thus, by setting $C = \max\{\beta(x^2 + \beta), 4\}$, we have that for $j \le t$ we have $b_j^2 \ge C \log(n)/n \ge s^2 C \log(n)/c^2 n$. Therefore, by Lemmas 8 and 9, with high probability the value of $T_j^{RF+}$ on any active column is larger than $T_j^{RF+}$ on any inactive column, so that *ReFACTor+* correctly identifies the active columns and the theorem follows. □

**Theorem 5.** *Make the same assumptions as in Theorem 4. For every fixed $\epsilon > 0$, with high probability we have for the relative improvement in MSE*

$$\frac{\left|\left|\hat{X}_1 - X\right|\right|_F^2 - \left|\left|\hat{X}_t^{RF+} - X\right|\right|_F^2}{||X||_F^2} \ge 1 - \frac{t + \log n}{n}(1 + \epsilon) .$$

**Proof:** The proof is identical to the proof of Theorem 1. □

Finally, we prove the following:

**Theorem 6.** *Assume that $x > \sqrt{1 + 2\sqrt{\beta}}$. There exists a constant $C_0$ such that if*

$$t \le C_0 \frac{n}{\log n} \tag{5}$$

*then with high probability*

$$\left|\left|\hat{X}_t^{RF+} - X\right|\right|_F^2 \le \left|\left|\hat{X}_1 - X\right|\right|_F^2 .$$

**Proof:** Let $R^+, R^-, R^{++}, R^{+-}, R^{-+}, R^{--}$ and $\Delta(R)$ be defined analogously to the definition in the proof of Theorem 3 (but with *ReFACTor+* instead of *ReFACTor*). We need to show that $\Delta(R^{+-}) + \Delta(R^{--}) < 0$ with high probability.

Using the exact same arguments as in Theorem 3, we can show that there exists $C_1 > 0$ so that with high probability

$$\Delta(R^{--}) = -y^2 \cdot \sum_{j \in R^{--}} v_j^2 \le -\frac{x^2 s^2 C_1}{2}.$$

We now bound from above the loss from false negatives. Recall that $\Delta(R^{+-}) = x^2 \sum_{j \in R^{+-}} b_j^2$. Denote $T = (2\beta y^2 s^2 \log n)/n$. Let $C = \max\{\beta(x^2 + \beta), 4\}$, and let $K = \left\{j \mid b_j^2 \ge (s^2 C \log n)/(c^2 n)\right\}$. By Lemmas 8 and 9, with high probability, for each $j \in R^-$ we have $T_j^{RF+} \le T$, and for each $j \in K$ with high probability $T_j^{RF+} \ge T$. Thus, with high probability $R^{+-} \cap K = \phi$. Thus

$$\Delta(R^{+-}) \le |R^{+-}| \frac{x^2 s^2 C \log(n)}{c^2 n} \le \frac{C_0 C x^2 s^2}{c^2},$$

using $t \le (C_0 n)/\log n$. By Lemma 4, with high probability $c^2 \ge 1/2$, and thus

$$\Delta(R^{+-}) \le 2 C_0 C x^2 s^2$$

Putting it all together, with high probability and for $C_0$ chosen to be a small enough constant

$$\Delta(R^{+-}) + \Delta(R^{--}) \le x^2 s^2 \left(2 C_0 C - \frac{C_1}{2}\right) < 0 .$$

Note that in this case $C_0$ is a function of $x$, and is decreasing when $x$ increases. □

# 2 DNA methylation

We now describe the real data experiment in full. For evaluating the performance of the different methods, we obtained from the Gene Expression Omnibus (GEO) database data that were studied in an association study of DNA methylation with rheumatoid arthritis (RA; GEO accession number GSE42861). We repeated the quality control procedure for the data applied in two recently published works on the same data [3,4]. Specifically, we filtered out sites with mean value higher than 0.8 or lower than 0.2, and we excluded three outlier samples. In total, we had methylation levels in a set of 103,638 sites for 686 individuals available for the analysis. We adjusted the data covariates (age, sex, smoking, and batch information), by fitting a linear regression model for each site as the explained variable using the covariates and using the residuals of the model as the adjusted methylation levels of this site. Then, each site was mean-centered.

We then conducted an association test for each adjusted site in the data using a logistic regression model with the disease status as the explained variable. Prior to fitting the model, for each method we adjusted the data for the signal it captured, by fitting a linear regression model for each covariate-adjusted site as the explained variable using the principal components of the specific method.

# 3 Comparison of *ReFACTor*, *JL* and TSVD

This sections contains the details of simulation testing the performance of *ReFACTor*, TSVD and *JL* on various parameters.

**Reproducible research.** The results in this paper are fully reproducible. Following publication, the code will be deposited in a permanent code repository. The reader can experiment with the scripts to generate additional figures in additional scenarios omitted for space considerations.

## 3.1 Gaussian noise, various parameters.

In this subsection, we examine the behaviour of these algorithms, when the noise is Gaussian, as in the case in the paper.

### 3.1.1 Low $r$ ($r = 1$).

We first check the performance on a low rank matrix ($r = 1$). In Figure 22, simulations test the performance of *ReFACTor*, TSVD and *JL* on a $200 \times 200$ matrix of Gaussian noise, with $r = 1$. The number of active columns, $t$, is varied, and performance is measured by the MSE of the estimated matrix, averaged across 50 runs. The signal strength, $x$, is changed between simulations. Note that $x = 1.73$ is the threshold in Theorems 1 and 3, above which *ReFACTor* has superior MSE.

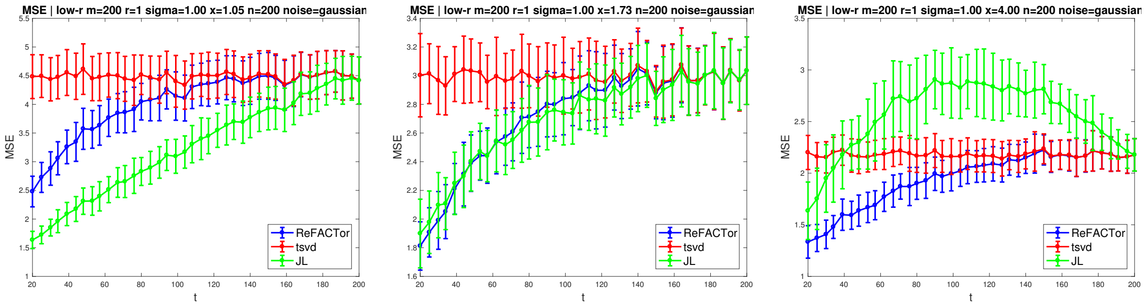


(a) x=1.05 (b) x=1.73 (c) x=4.00

Figure 1: Varying $t$, $r = 1, m = 200, n = 200$, Gaussian noise.

In Figure 23, we instead vary the signal $x$, for a fixed number of active columns $t$, which varies across figures.

Figure 24 varies the number of columns $n$, while fixing $t$ and $x$.

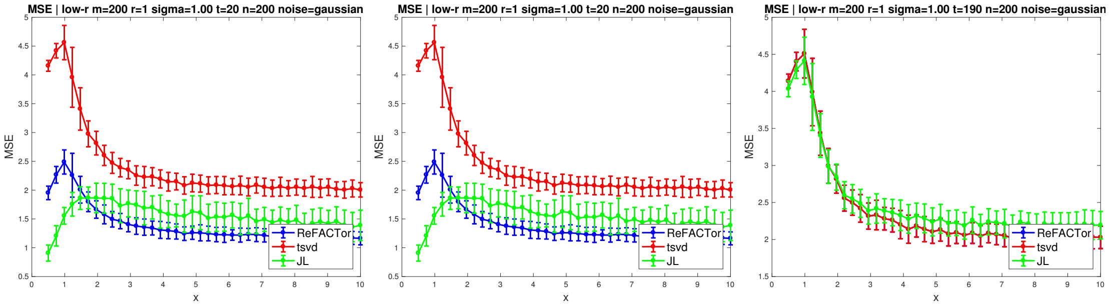


(a) $t = 20$ (b) $t = 100$ (c) $t = 190$

Figure 2: Varying $x$, $r = 1, m = 200, n = 200$, Gaussian noise.

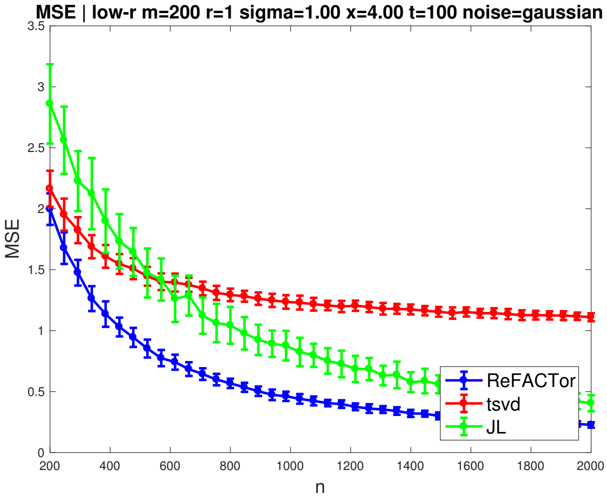


Figure 3: Varying $n$, $r = 1, x = 4, t = 100, m = 200, n = 200$, Gaussian noise.

### 3.1.2 Medium $r$ ($r = 5$).

The same analyses are performed for a medium $r$, $r = 5$.

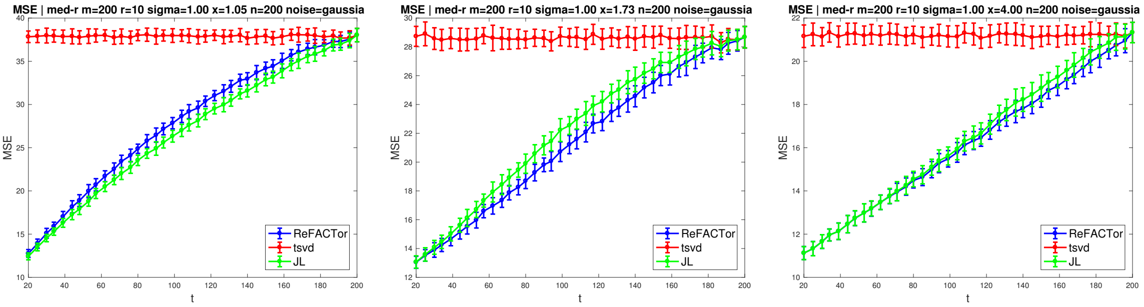


(a) $x = 1.05$ (b) $x = 1.73$ (c) $x = 4.0$

Figure 4: Varying $t$, $r = 10, m = 200, n = 200$, Gaussian noise.

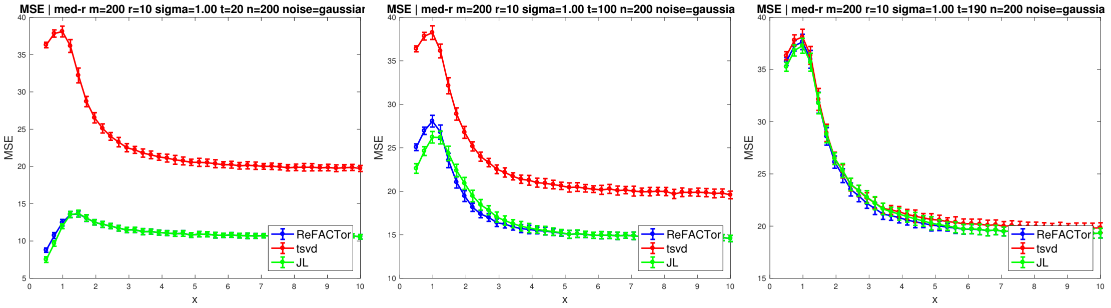


(a) $t = 20$ (b) $t = 100$ (c) $t = 190$

Figure 5: Varying $x$, $r = 10, m = 200, n = 200$, Gaussian noise.

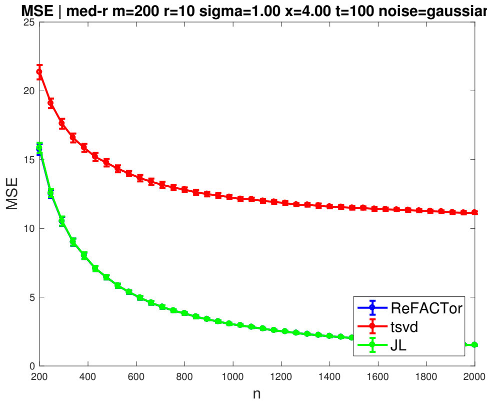


Figure 6: Varying $n$, $r = 10, x = 4, t = 100, m = 200, n = 200$, Gaussian noise.

### 3.1.3 High $r$ ($r = 40$).

The same analyses are performed for a medium $r$, $r = 40$.

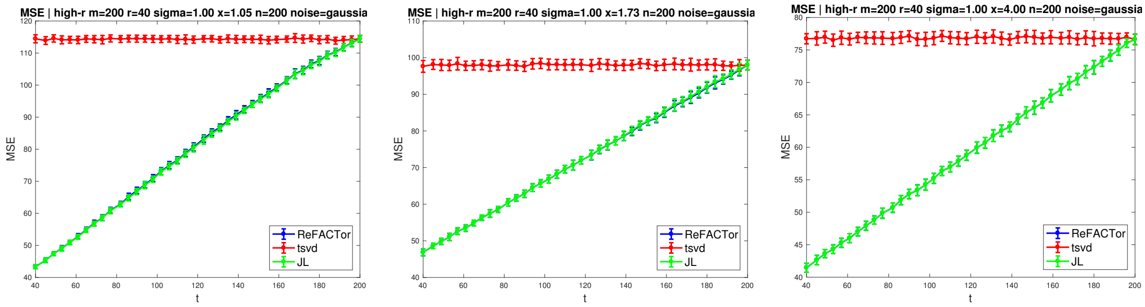


(a) $x = 1.05$ (b) $x = 1.73$ (c) $x = 4.0$

Figure 7: Varying $t$, $r = 40, m = 200, n = 200$, Gaussian noise.

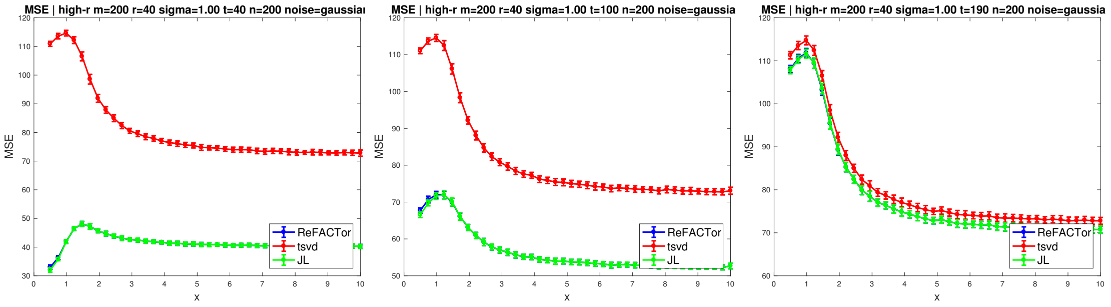


(a) $t = 40$

(b) $t = 100$

(c) $t = 190$

Figure 8: Varying $x$, $r = 40, m = 200, n = 200$, Gaussian noise.

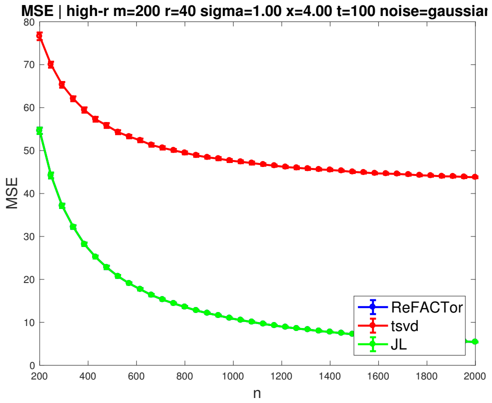


Figure 9: Varying $n$, $r = 40, x = 4, t = 100, m = 200, n = 200$, Gaussian noise.

#### 3.1.4 Matrix dimensions, $\beta = m/n = 1/2$.

Finally, we test the effect of a non-square matrix on the results. The same analyses are performed, for $\beta = m/n = 1/2$, and $r = 5$.

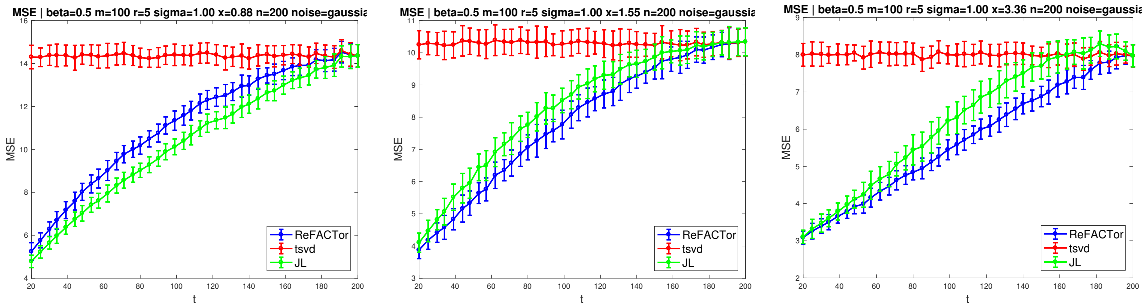


(a) $x = 0.88$

(b) $x = 1.55$

(c) $x = 3.66$

Figure 10: Varying $t$, $r = 5, m = 100, n = 200$, Gaussian noise.

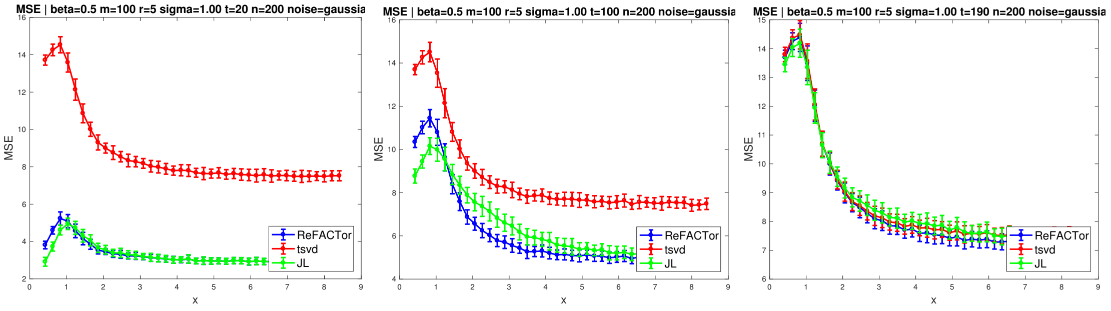


(a) $t = 20$ (b) $t = 100$ (c) $t = 190$

Figure 11: Varying $x$, $r = 5, m = 100, n = 200$, Gaussian noise.

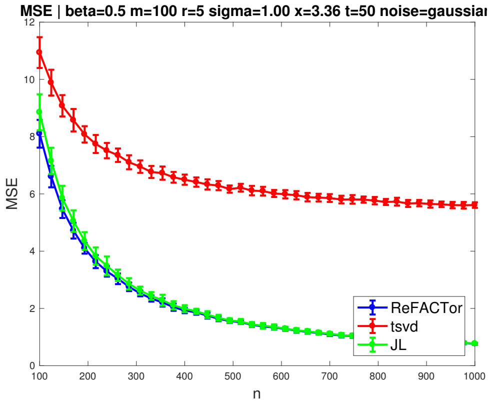


Figure 12: Varying $n$, $r = 5, x = 3.36, t = 50, m = 100, n = 200$, Gaussian noise.

## 3.2 Various Distributions

In this subsection, we see the effect of various noise distributions on the performance of the compared algorithms. We analyze the following distributions:

1. Gaussian
2. Uniform
3. Student's $t$ distribution, with 6 degrees of freedom

The analyses are the same as in Section 4.1, with a common $r = 5$.

### 3.2.1 Gaussian

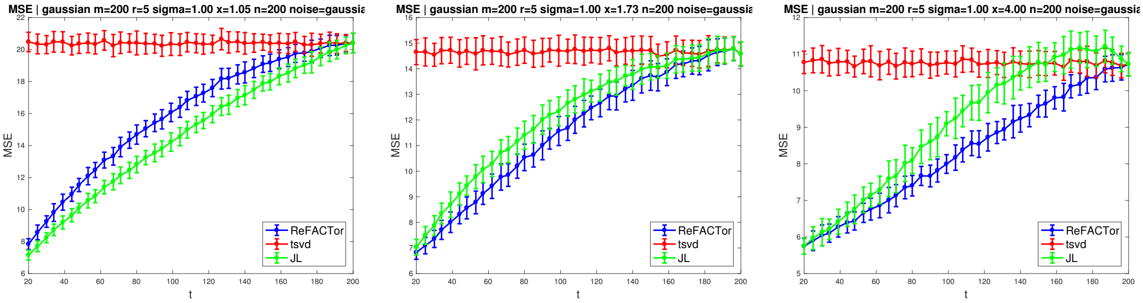


(a) x=1.05 (b) x=1.73 (c) x=4.00

Figure 13: Varying $t$, $r = 5, m = 200, n = 200$, Gaussian noise.

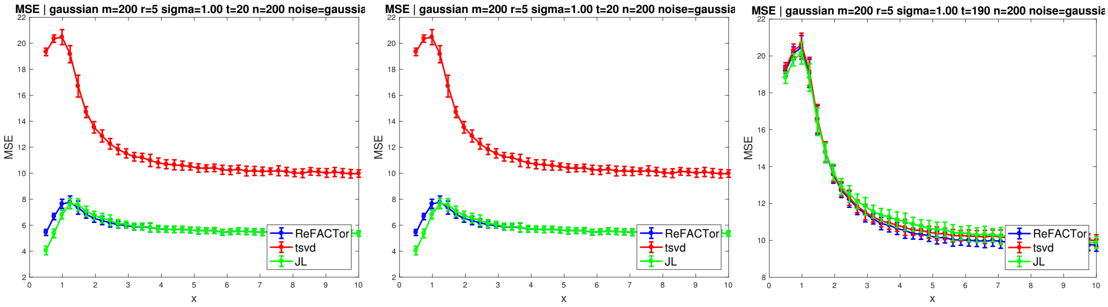


(a) $t = 20$ (b) $t = 100$ (c) $t = 190$

Figure 14: Varying $x$, $r = 5, m = 200, n = 200$, Gaussian noise.

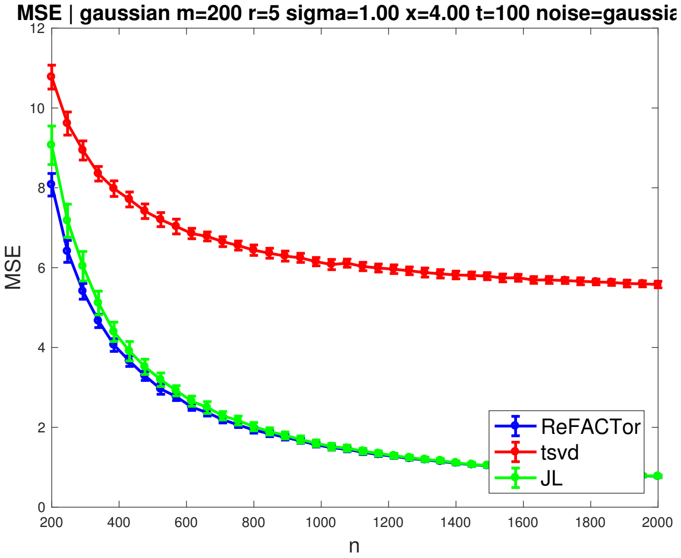


Figure 15: Varying $n$, $r = 5, x = 4, t = 100, m = 200, n = 200$, Gaussian noise.

### 3.2.2 Uniform

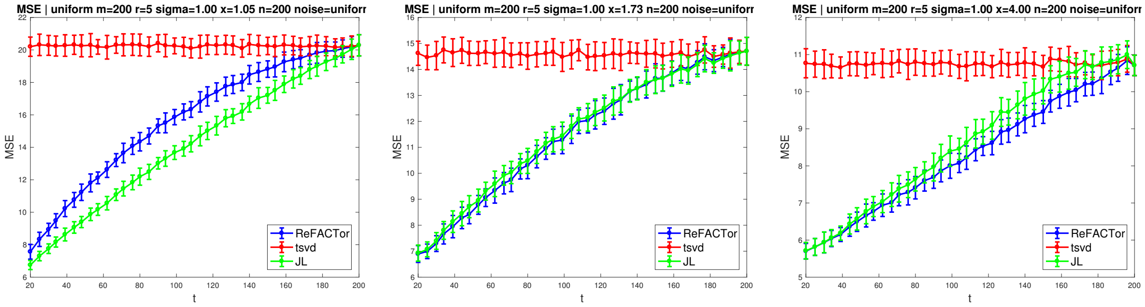


(a) x=1.05 (b) x=1.73 (c) x=4.00

Figure 16: Varying $t$, $r = 5, m = 200, n = 200$, uniform noise.

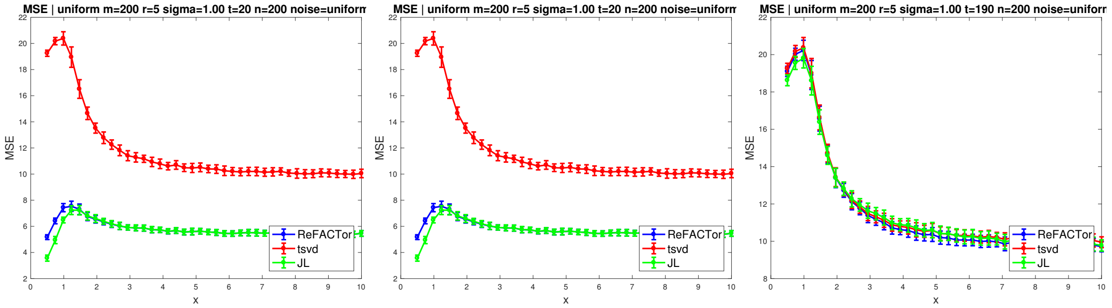


(a) $t = 20$ (b) $t = 100$ (c) $t = 190$

Figure 17: Varying $x$, $r = 5, m = 200, n = 200$, uniform noise.

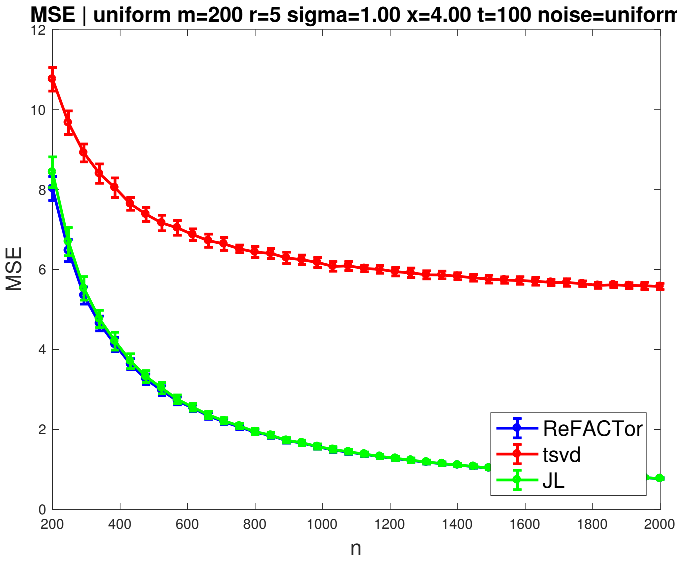


Figure 18: Varying $n$, $r = 5, x = 4, t = 100, m = 200, n = 200$, uniform noise.

### 3.2.3 Student's $t$

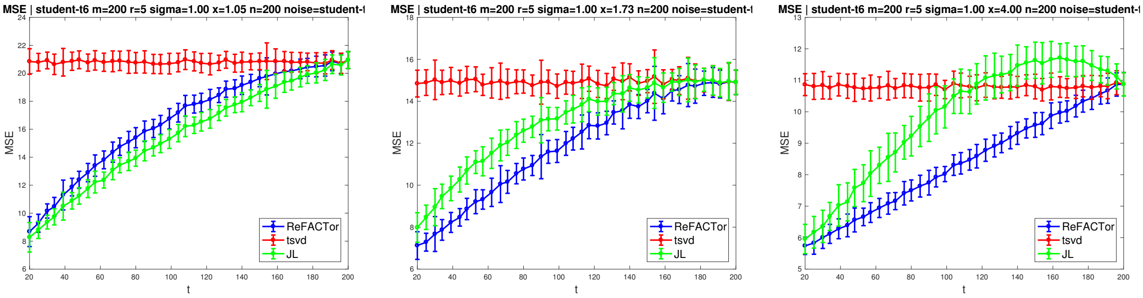


(a) x=1.05 (b) x=1.73 (c) x=4.00

Figure 19: Varying $t$, $r = 5, m = 200, n = 200$, student-t6 noise.

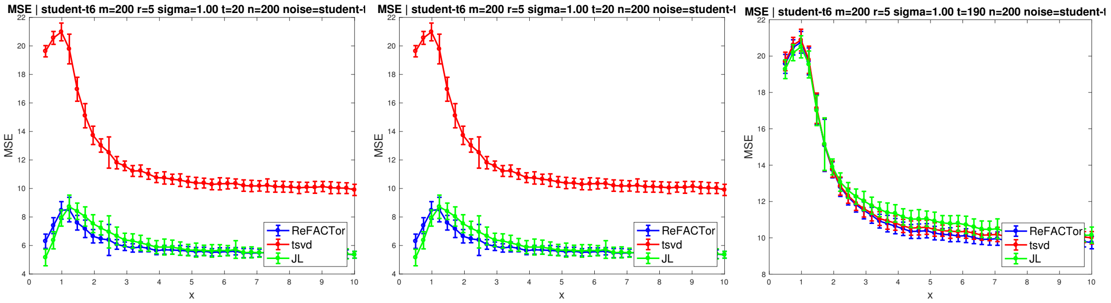


(a) $t = 20$ (b) $t = 100$ (c) $t = 190$

Figure 20: Varying $x$, $r = 5, m = 200, n = 200$, student-t6 noise.

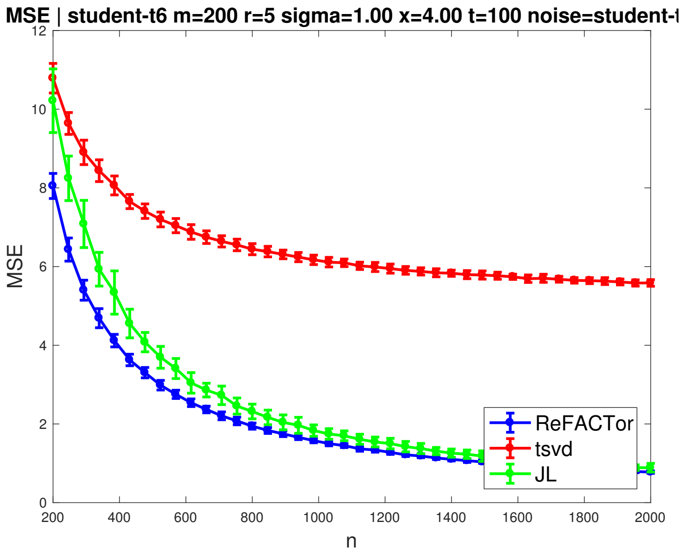


Figure 21: Varying $n$, $r = 5, x = 4, t = 100, m = 200, n = 200$, student-t6 noise.

# 4 Comparison of *ReFACTor*, *ReFACTor*$^*$, *ReFACTor+*, *JL*, *JL*$^*$ and TSVD

In these sections, we additionally examine the performance of the studied variants, *ReFACTor*$^*$, *ReFACTor+* and *JL*$^*$. We repeat all the analyses in Section 3, omitting standard errors for clarity of presentation.

## 4.1 Gaussian noise, various parameters.

In this subsection, we examine the behaviour of these algorithms, when the noise is Gaussian, as in the case in the paper.

### 4.1.1 Low $r$ ($r = 1$).

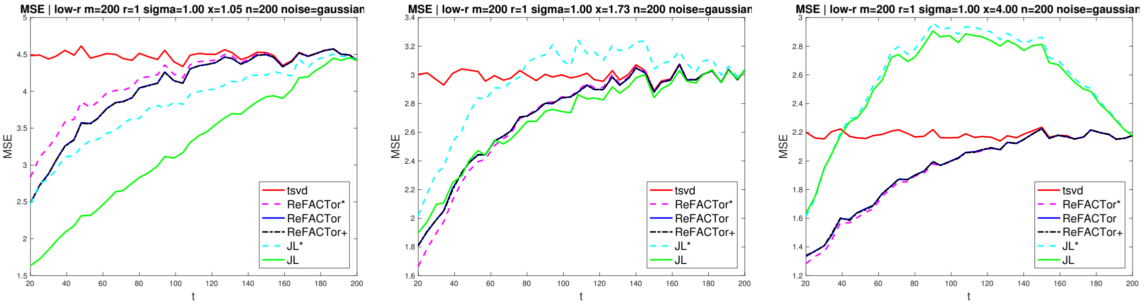


(a) x=1.05 (b) x=1.73 (c) x=4.00

Figure 22: Varying $t$, $r = 1, m = 200, n = 200$, Gaussian noise.

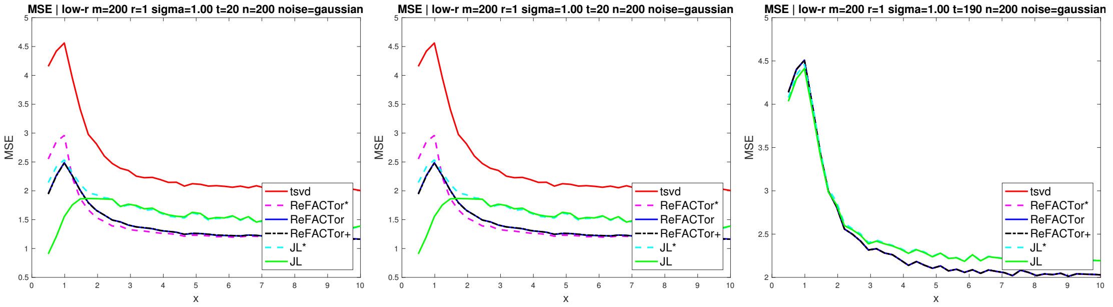


(a) $t = 20$ (b) $t = 100$ (c) $t = 190$

Figure 23: Varying $x$, $r = 1, m = 200, n = 200$, Gaussian noise.

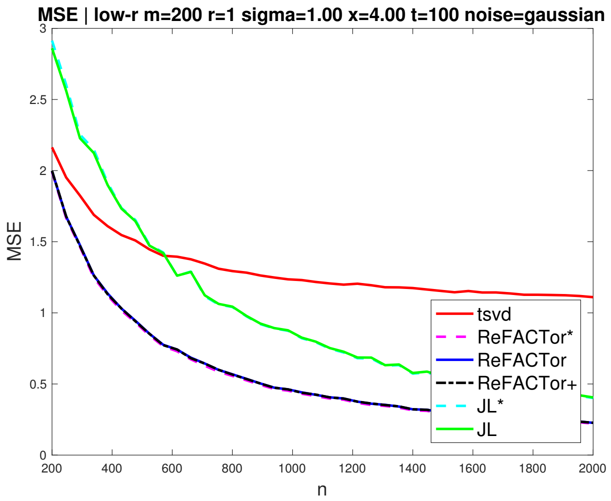


Figure 24: Varying $n$, $r = 1, x = 4, t = 100, m = 200, n = 200$, Gaussian noise.

### 4.1.2 Medium $r$ ($r = 5$).

The same analyses are performed for a medium $r$, $r = 5$.

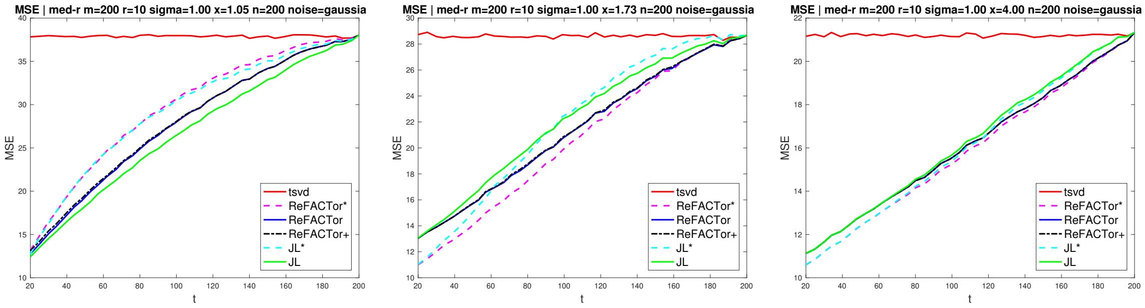


(a) $x = 1.05$ (b) $x = 1.73$ (c) $x = 4.0$

Figure 25: Varying $t$, $r = 10, m = 200, n = 200$, Gaussian noise.

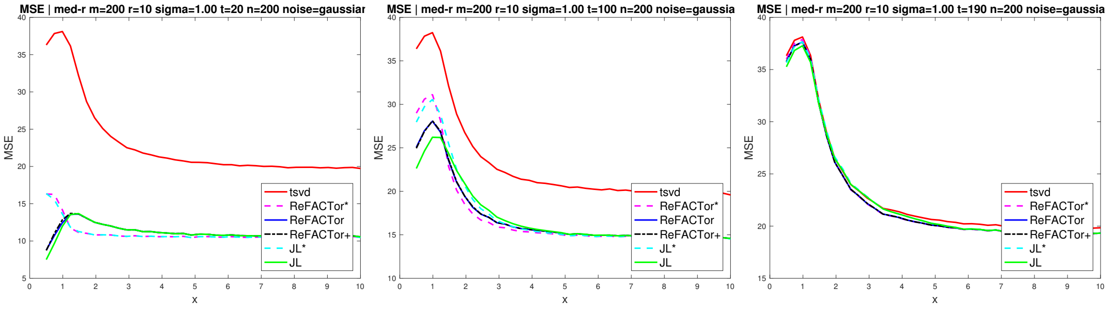


(a) $t = 20$ (b) $t = 100$ (c) $t = 190$

Figure 26: Varying $x$, $r = 10, m = 200, n = 200$, Gaussian noise.

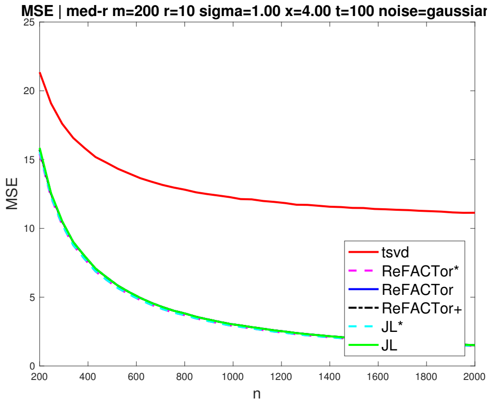


Figure 27: Varying $n$, $r = 10, x = 4, t = 100, m = 200, n = 200$, Gaussian noise.

### 4.1.3 High $r$ ($r = 40$).

The same analyses are performed for a medium $r$, $r = 40$.

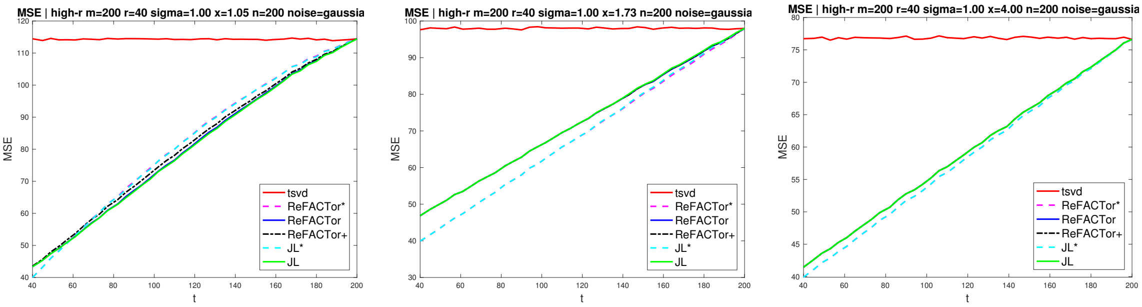


(a) $x = 1.05$ (b) $x = 1.73$ (c) $x = 4.0$

Figure 28: Varying $t$, $r = 40, m = 200, n = 200$, Gaussian noise.

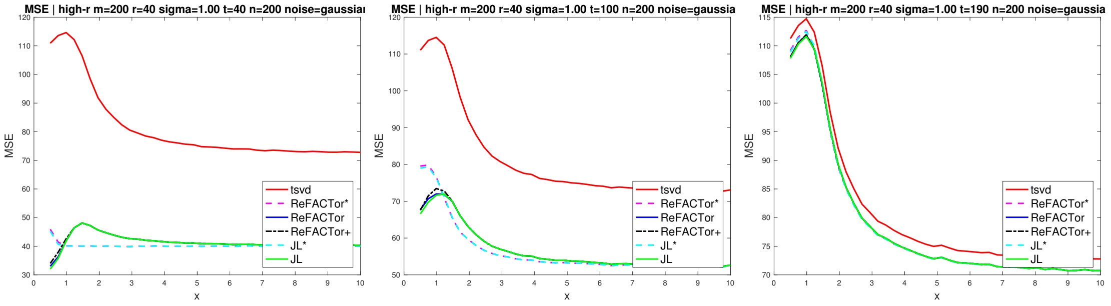


(a) $t = 40$ (b) $t = 100$ (c) $t = 190$

Figure 29: Varying $x$, $r = 40, m = 200, n = 200$, Gaussian noise.

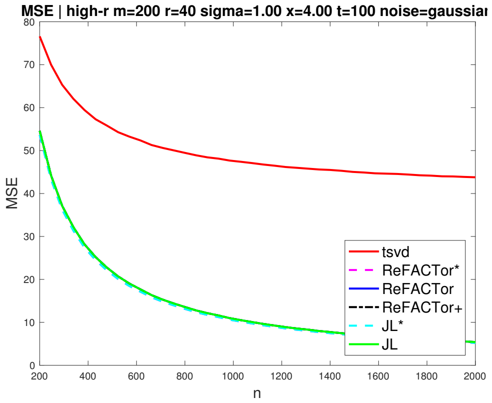


Figure 30: Varying $n$, $r = 40, x = 4, t = 100, m = 200, n = 200$, Gaussian noise.

### 4.1.4 Matrix dimensions, $\beta = m/n = 1/2$.

Finally, we test the effect of a non-square matrix on the results. The same analyses are performed, for $\beta = m/n = 1/2$, and $r = 5$.

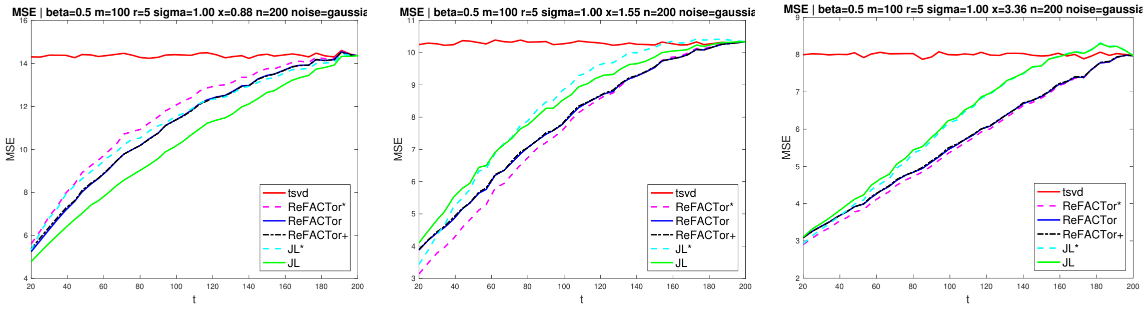


(a) $x = 0.88$ (b) $x = 1.55$ (c) $x = 3.66$

Figure 31: Varying $t$, $r = 5, m = 100, n = 200$, Gaussian noise.

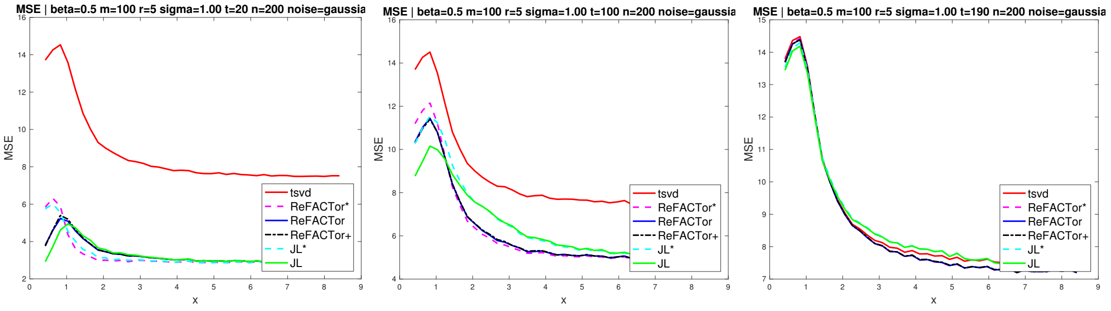


(a) $t = 20$ (b) $t = 100$ (c) $t = 190$

Figure 32: Varying $x$, $r = 5, m = 100, n = 200$, Gaussian noise.

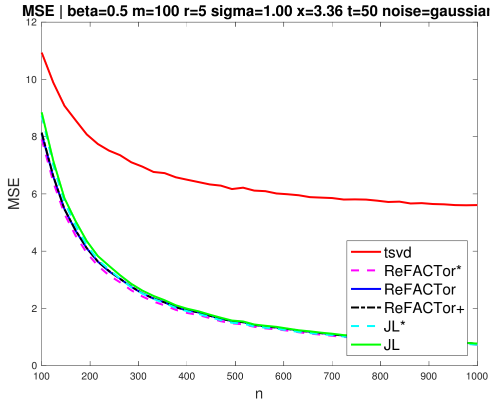


Figure 33: Varying $n$, $r = 5, x = 3.36, t = 50, m = 100, n = 200$, Gaussian noise.

## 4.2 Various Distributions

In this subsection, we see the effect of various noise distribution on the performance of the compared algorithms. We analyze the following distributions:

1. Gaussian
2. Uniform
3. Student's $t$ distribution, with 6 degrees of freedom

The analyses are the same as in Section 4.1, with a common $r = 5$.

### 4.2.1 Gaussian

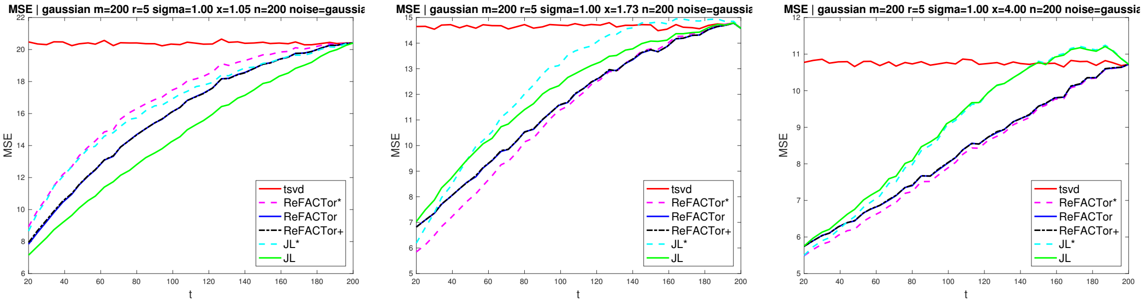


(a) x=1.05 (b) x=1.73 (c) x=4.00

Figure 34: Varying $t$, $r = 5, m = 200, n = 200$, Gaussian noise.

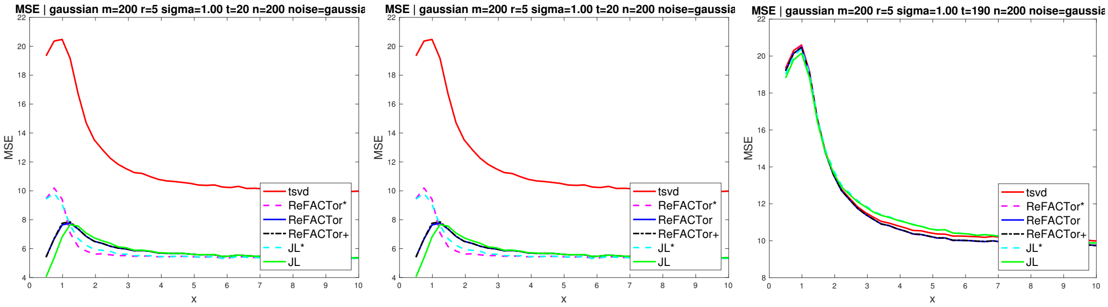


(a) $t = 20$ (b) $t = 100$ (c) $t = 190$

Figure 35: Varying $x$, $r = 5, m = 200, n = 200$, Gaussian noise.

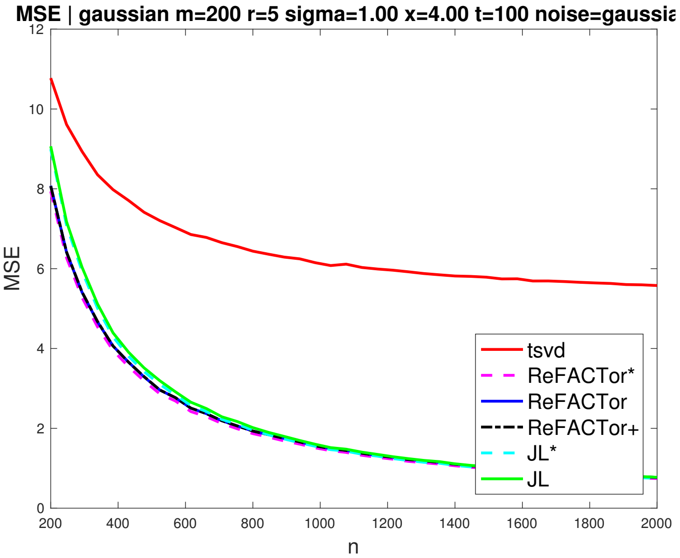


Figure 36: Varying $n$, $r = 5, x = 4, t = 100, m = 200, n = 200$, Gaussian noise.

### 4.2.2 Uniform

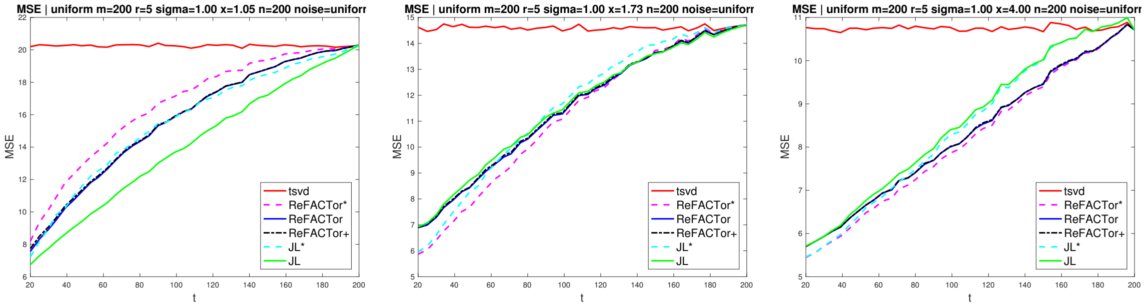


(a) x=1.05 (b) x=1.73 (c) x=4.00

Figure 37: Varying $t$, $r = 5, m = 200, n = 200$, uniform noise.

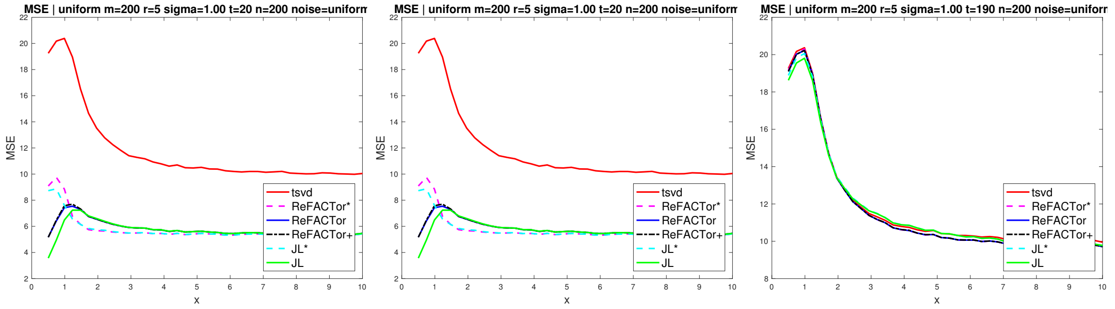


(a) $t = 20$ (b) $t = 100$ (c) $t = 190$

Figure 38: Varying $x$, $r = 5, m = 200, n = 200$, uniform noise.

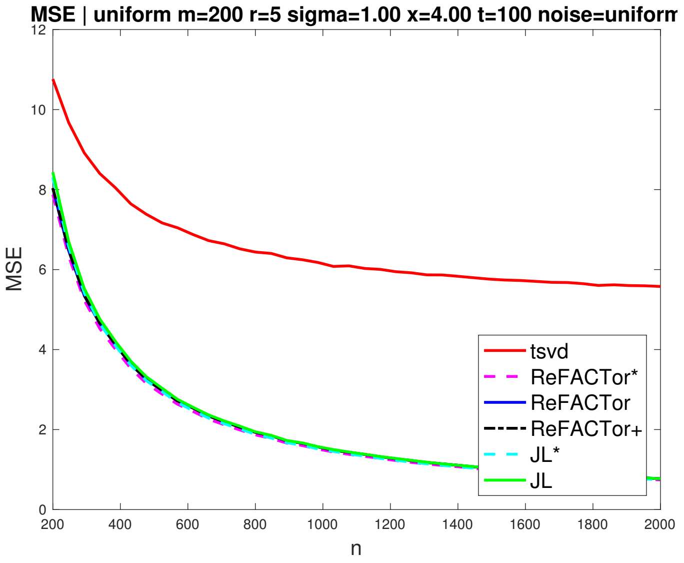


Figure 39: Varying $n$, $r = 5, x = 4, t = 100, m = 200, n = 200$, uniform noise.

### 4.2.3 Student's $t$

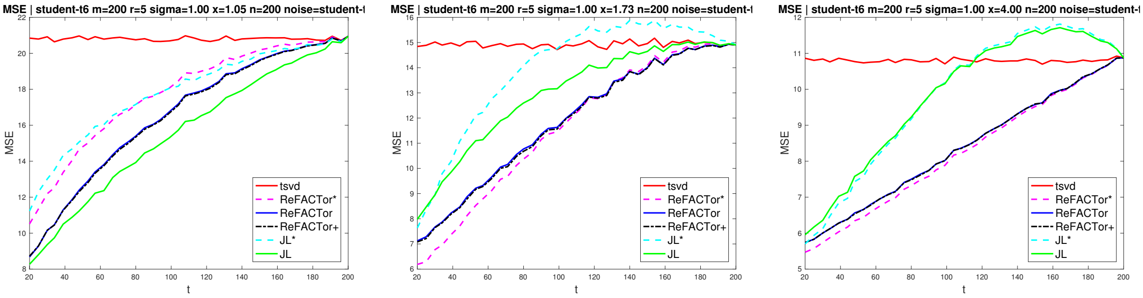


(a) x=1.05 (b) x=1.73 (c) x=4.00

Figure 40: Varying $t$, $r = 5, m = 200, n = 200$, student-t6 noise.

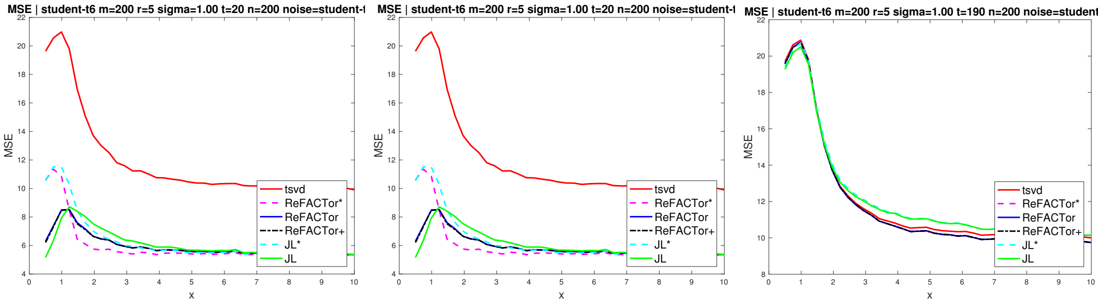


(a) $t = 20$ (b) $t = 100$ (c) $t = 190$

Figure 41: Varying $x$, $r = 5, m = 200, n = 200$, student-t6 noise.

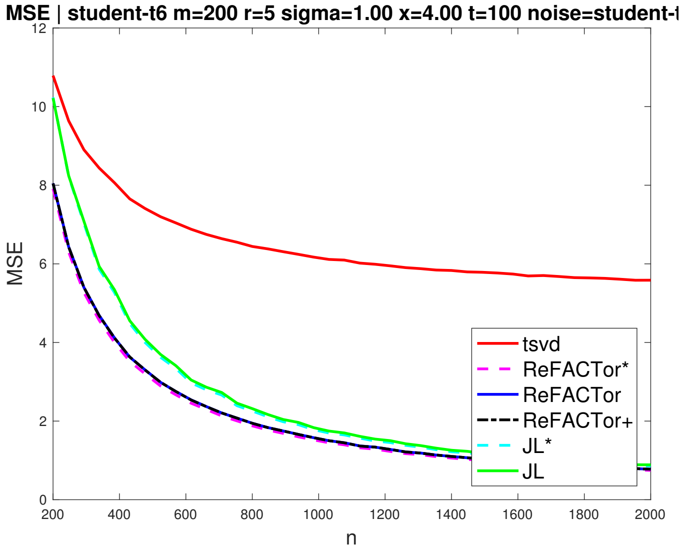


Figure 42: Varying $n$, $r = 5, x = 4, t = 100, m = 200, n = 200$, student-t6 noise.

# References

[1] Kenneth R Davidson and Stanislaw J Szarek. Local operator theory, random matrices and banach spaces. *Handbook of the geometry of Banach spaces*, 1(317-366):131, 2001.

[2] William Feller. *An introduction to probability theory and its applications*, volume 2. John Wiley & Sons, 2008.

[3] Elior Rahmani, Noah Zaitlen, Yael Baran, Celeste Eng, Donglei Hu, Joshua Galanter, Sam Oh, Esteban G Burchard, Eleazar Eskin, James Zou, et al. Sparse pca corrects for cell type heterogeneity in epigenome-wide association studies. *Nature methods*, 13(5):443–445, 2016.

[4] James Zou, Christoph Lippert, David Heckerman, Martin Aryee, and Jennifer Listgarten. Epigenome-wide association studies without the need for cell-type composition. *Nature methods*, 11(3):309–311, 2014.
